# Supplementary material for: A Learnability Analysis on Neuro-Symbolic Learning
Source: arXiv:2503.16797 source file (2025-03-21)
Supplement: Supplementary file 1 [file appendix.example.tex]

\section{Ensemble of Unlearnable NeSy Tasks}\label{appendix: ensemble example}
